# Supplementary material for: Asynchronous Multi Agent Active Search
Source: arXiv:2006.14718 source file (2020-06-25)
Supplement: Supplementary file 1 [file 7-appendices.tex]

% !TEX root = 18ICML_PhaseInit.tex
%%%%%%%%%%%%%%%%%%%%%%%%%%%%%%
%

%\appendices

\section{Proof of \fref{thm:TS}}

????
